# Supplementary material for: Investigating Unusual H$\alpha$ Features towards the Scutum Supershell
Source: arXiv:2410.15712 source file (2024-10-21)
Supplement: Supplementary file 1 [file source_appendix.tex]

\subsection{Atomic Hydrogen Supershells}

\autoref{tab:obGSH}  lists the Galactic supershells so far identified with total energy above $10^{52}$\,erg taken from various references as listed. 

\begin{table}
    \caption{List of Galactic supershells (GSH) with total energy (E) above $10^{52}$\,erg, age, mass, and distance (D). Data are taken from \cite{2019yCat..36240043S}, $\ast$ \cite{2001A&A...374..682E}, $\dagger$  \cite{2015AJ....149..189S}, $\star$ \cite{2006ApJ...638..196M}, $\blacklozenge$ \cite{2011ApJ...741...85D}, and $\blacktriangle$ \cite{2014A&A...562A..69K}. The Scutum Supershell is highlighted in boldface.
    }
    \centering
    % \small
    \begin{tabular}{lcccc}
    \toprule
    GSH & log(E) & Age & Mass & D \\
    & (erg) & (Myr) & ($10^{4}$ M$_\odot$) & (kpc) \\ \hline
    016-01+71 & 52.4 & ~ & 5.8 & 6.3 \\ 
    \textbf{018-04+44} & \textbf{52.0} &  & \textbf{62} & \textbf{3.3}\\ 
    022+01+139 & 53.0 & ~ & 6.4 & 9.5 \\ 
    029+00+133 & 52.6 & ~ & 6.3 & 8.7 \\ 
    033+06-49 & 52.9 & ~ & 6.8 & 22 \\ 
    034-06+65 & 52.1 & ~ & 6 & 4.6 \\ 
    041+01+27 & 52.9 & ~ & 6.7 & 2 \\ 
    046-01+83 & 52.0 & ~ & 6 & 6.9 \\ 
    052+07+39 & 52.1 & ~ & 6 & 3.1 \\ 
    052+02-071 $\dagger$  & 52 & ~ & ~ & ~ \\ 
    057+01-33 & 53.6 & ~ & 7 & 13.8 \\ 
    061+00+51 & 52.1 & ~ & 5.7 & 4.8 \\ % The H I supershell GS061+00+51 and its neighbours 
    064-01-97 & 53.8 & ~ & 7.1 & 16.9 \\
    071+06-135 & 54.2 & ~ & 7.8 & 21.6 \\ 
    075-01+39 & 52.9 & ~ & 6.2 & 2.6 \\ 
    081-05-37 & 52.9 & ~ & 6.9 & 7.5 \\ 
    088+02-103 & 54.1 & ~ & 7.3 & 12.6 \\ 
    091-04-69 & 52.8 & ~ & 6.8 & 9 \\ 
    091+02-101 & 52.3 & ~ & 6.3 & 12.3 \\ 
    095+04-113 & 53.5 & ~ & 7.3 & 12.9 \\ 
    103+05-137 & 53.4 & ~ & 7 & 15.6 \\ 
    108-04-23 & 52.7 & ~ & 6.1 & 2.5 \\ 
    117-07-67 & 52.2 & ~ & 6 & 6.3 \\ 
    123+07-127 & 53.3 & ~ & 7.4 & 15.1 \\ 
    128+01-105 & 52.2 & ~ & 6.3 & 11.4 \\ 
    139-03-69 & 54.8 & ~ & 8.2 & 7.1 \\ 
    187+01+020 $\dagger$  & 52.0 & ~ & ~ & ~ \\ 
    20+05+23 & 52.2 & ~ & 6 & 4.8 \\ 
    223-02+35 & 52.6 & ~ & 6.6 & 3.5 \\ 
    224+03+75 & 53.4 & ~ & 7 & 7.6 \\ 
    242-03+37 & 54.2 & ~ & 7.5 & 3.6 \\ 
    242-03+37 $\star$ & 53.0 & 21 & 4.8 & 1.6 \\ %EVIDENCE FOR CHIMNEY BREAKOUT IN THE GALACTIC SUPERSHELL GSH 24203+37
    277+00+36 $\blacklozenge$ & 53.0 & >10 &  >100 & 6.5 \\ %Molecular Clouds in Supershells: A Case Study of Three Objects in the Walls of GSH 287+04-17 and GSH 277+00+36
    287+04-17 $\blacklozenge$ & 52.0 & >10 &  >100 & 2.6 \\ %Molecular Clouds in Supershells: A Case Study of Three Objects in the Walls of GSH 287+04-17 and GSH 277+00+36
  \hline
    \end{tabular}
    \label{tab:obGSH}
\end{table}

\subsection{Decomposing the WHAM H\texorpdfstring{$\alpha$}{} Spectra with {\tt GaussPy+}} \label{Gpy}

Here, we used the {\tt GaussPy+} package \citep{2019A&A...628A..78R,2015AJ....149..138L} to decompose the components of the WHAM H$\alpha$ spectra for the region shown in \autoref{V_l}.
{\tt GaussPy+} fits are shown in \autoref{fig:gausspy}% and \autoref{tab:gausp} 
for the eight spectral pixels shown in  \autoref{V_l}.
The {\tt GaussPy+} fitting decomposes each pixel's spectrum into typically five to six Gaussian components with one to two clearly dominant components. In the {\tt GaussPy+} process, we trained the smoothing parameter $\alpha$ using a wide region with boundaries $b=-8^\circ$\,to\,8$^\circ$ and $l=10^\circ$\,to\,24$^\circ$.
We trained with 250 spectra, resulting in an $\alpha$ value of 4.68.
Due to the spectral  resolution of WHAM, we have set a minimum FWHM of 12\,km\,s$^{-1}$ (6 channels) for each Gaussian component. 

\begin{figure*}
    \centering 
    \includegraphics[width=\textwidth]{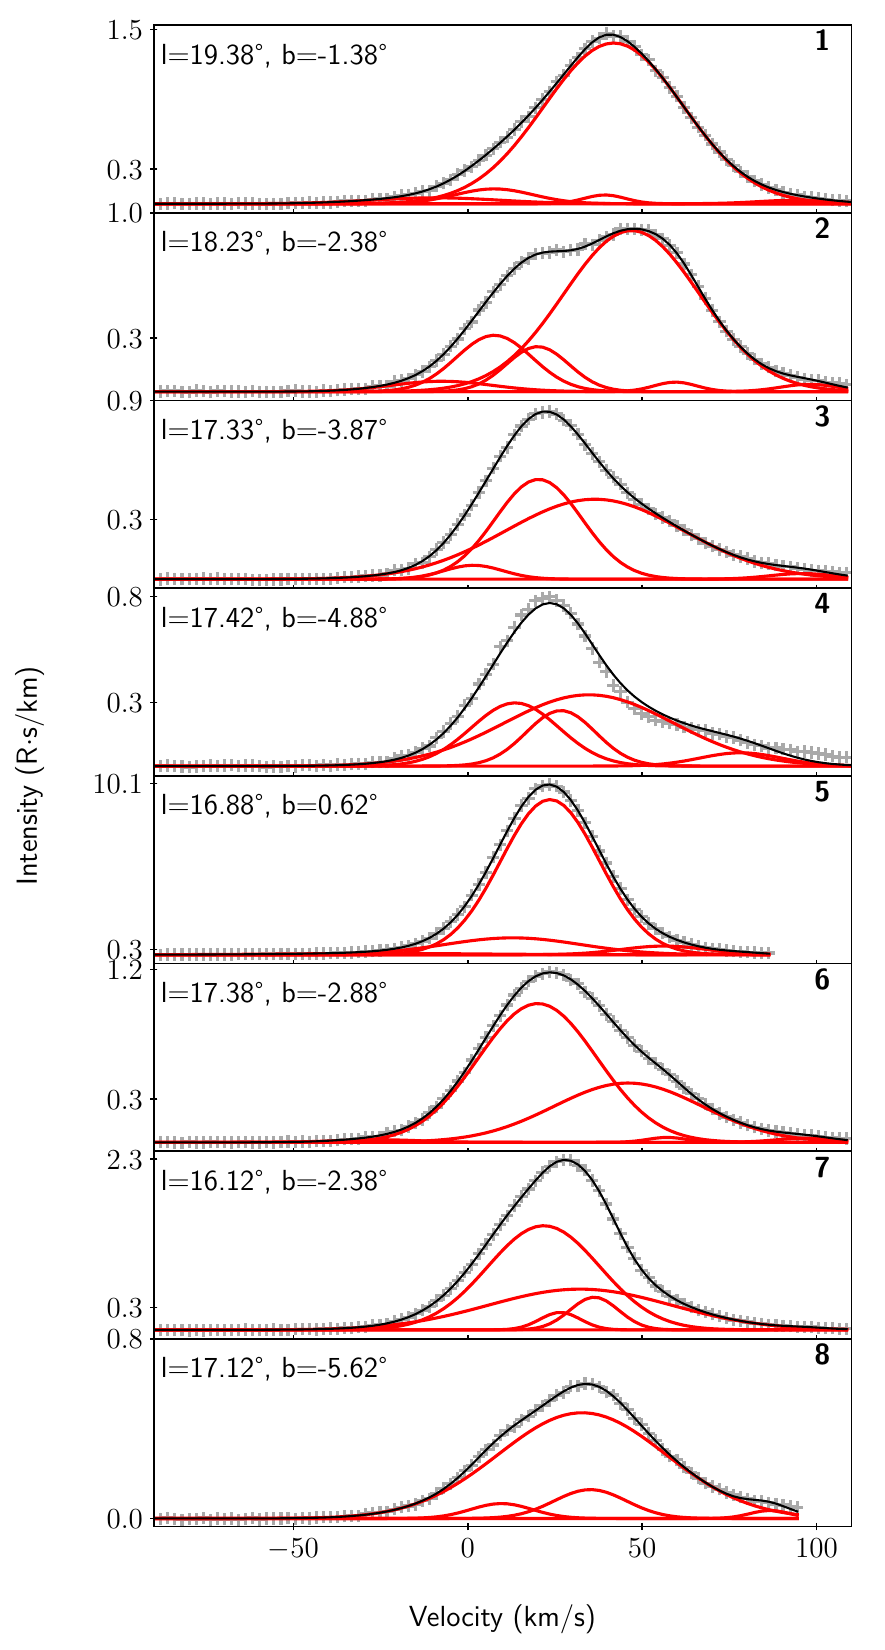} 
    \caption{WHAM H$\alpha$ spectra from  \citet{1998PASA...15...14R} for the eight pixels shown in \autoref{V_l}. The {\tt GaussPy+} fit results are shown as red lines for the individual components with the dashed black line showing the total. %The number of Gaussian components (\# 
    }
    \label{fig:gausspy}
\end{figure*}

\subsection{Spectral Type of O stars }
\red{
OB Stars from \citet{2003AJ....125.2531R} were used, employing {\tt Astropy} and {\tt SIMBAD} to determine the spectral type and distance of each star.
Removing any duplicated stars in the catalogue, a list of O-type stars are in \autoref{tab:star_photo_fesc}.
The distance and its error are found using Gaia DR3 parallax \cite{2020yCat.1350....0G}.
We measure $r$ the distance to the bow-shock, using the coordinates Galactic longitude of 17.5$^{\circ}$ and Galactic latitude of $-$5.5$^{\circ}$ showing at \autoref{fig:HII_region}.
\autoref{tab:star_photo_fesc2} shows stars with spectral type `OB', showing their distance and their magnitude.
}

\begin{onecolumn}
\begin{longtable}{lcccccccc}
\caption{\red{ A list of O-type stars  from \citet{2003AJ....125.2531R} were their spectral type is found using {\tt Astropy} and {\tt SIMBAD}, and they are limited to the region between $15.5^\circ \leq l \leq 21^\circ$ and  $-5^\circ \leq b \leq 5^\circ$. the stars magnitude  (mag) is listed from \cite{2003AJ....125.2531R} (mag). The distance and using Gaia DR3 parallax \cite{2020yCat.1350....0G} is showed. The distance to the bow-shock is $r$, measured with coordinates given as GL=17.5$^{\circ}$ and GB=$-$5.5$^{\circ}$ \autoref{fig:HII_region}.  Galactic longitude and latitude are $l$ and $b$, respectively. }}  \label{tab:star_photo_fesc} \\
\toprule

                Name &   $\mathrm{mag}$&  $ {l}$  &    $ {b}$  & Dist &     S(type) &  S(type) reference &     $r$ &\\
                     &  &  (deg)    & (deg)  & (pc$\pm$5\% )   &       &        & (pc)   &  \\
\midrule
\endfirsthead

\toprule
              Name &   $\mathrm{mag}$  &  $ {l}$  &    $ {b}$  &     Dist &     S(type) &  S(type)reference &     $r$ &      \\
                     &   & (deg)    & (deg)  &  (pc)$\pm$5\%    &       &        & (pc) & \\
\midrule
\endhead
\midrule
\multicolumn{8}{r}{{Continued on next page}} \\
\midrule
\endfoot

\bottomrule
\endlastfoot
LS  IV -15   42 & 10.9 & 15.70 & -0.06 & 2877.7 &           O8.5V+O8.5V & a&         629.8 \\
LS  IV -13    3 & 11.6 & 15.88 &  4.23 & 2125.8 &             ON6V((f)) & a&         195.9 \\
      HD 168444 &  8.8 & 16.20 & -0.01 & 1542.7 &            O9.5/B0Iab & c&         796.5 \\
      V* QR Ser &  9.2 & 16.81 &  0.67 & 2078.1 &     O9.5III+B3-5V/III & h&         307.9 \\
    V* V479 Sct & 12.0 & 16.88 & -1.29 & 2040.8 &            ON6V((f))z & a&         319.0 \\
    BD-14  5040 & 10.8 & 16.90 & -1.12 & 1716.7 &         O5.5V(n)((f)) & a&         614.5 \\
LS  IV -13   14 & 11.0 & 16.91 &  0.85 & 1830.1 &                   O9V & g&         512.6 \\
      HD 168075 &  8.8 & 16.94 &  0.84 & 1682.0 &          O7V(n)((f))z & b&         651.1 \\
    BD-13  4930 &  9.4 & 16.94 &  0.77 & 1786.0 &                 O9.7V & g&         554.6 \\
    BD-13  4928 & 10.1 & 16.97 &  0.82 & 1692.0 &              O9.7IVnn & g&         641.8 \\
      HD 168137 &  9.5 & 16.97 &  0.76 & 1881.1 &                  O8Vz & a&         467.9 \\
    BD-13  4929 & 10.4 & 16.98 &  0.82 & 1703.0 &      O7V+B0.5V+B0.5V: & h&         631.6 \\
    BD-13  4927 & 10.2 & 16.99 &  0.85 & 1758.7 &               O7II(f) & b&         578.7 \\
      HD 168504 & 10.0 & 17.03 &  0.35 & 1717.3 &             O7.5V(n)z & a&         625.1 \\
      HD 167330 &  9.6 & 17.66 &  2.16 & 1728.0 &          O9.5/B0Ia/ab & c&         590.3 \\
      HD 169727 &  9.9 & 17.99 & -0.82 & 2090.3 &                  O7II & d&         293.7 \\
    BD-12  5004 & 11.3 & 18.22 &  1.17 & 1874.7 &                  O9IV & d&         466.5 \\
    BD-12  4979 & 10.4 & 18.25 &  1.69 & 1912.0 &                 O9.5V & e&         423.3 \\
LS  IV -12   12 & 10.4 & 18.32 &  1.87 & 1829.1 &              O6V((f)) & a&         498.1 \\
      HD 168112 &  9.8 & 18.44 &  1.62 & 2006.0 &              O5III(f) & b&         341.8 \\
    BD-12  4984 & 10.0 & 18.53 &  1.77 & 2026.7 &                   O9V & o&         321.4 \\
      HD 168461 & 10.2 & 18.57 &  1.25 & 2125.4 &        O7.5V((f))Nstr & a&         259.3 \\
      HD 171589 &  8.3 & 18.64 & -3.09 & 1848.7 &             O7.5II(f) & b&         466.0 \\
    BD-12  5042 & 11.6 & 18.69 & -0.02 & 2181.0 &                  O9Ib & d&         272.8 \\
      V* RY Sct & 10.4 & 18.71 & -0.13 & 2106.1 &              O9.7Ibep & l&         309.3 \\
      HD 168206 &  9.1 & 18.91 &  1.75 & 2042.4 &         WC8+O8/9III/V & f&         311.3 \\
      HD 166734 &  8.4 & 18.92 &  3.63 & 1759.0 &              O7.5Iabf & b&         550.6 \\
    BD-11  4586 &  9.4 & 19.08 &  2.14 & 2009.6 &               O8Ib(f) & b&         332.6 \\
    BD-11  4620 & 10.2 & 19.15 &  0.67 & 2139.9 &                    O5 & o&         274.8 \\
    BD-12  5039 & 10.8 & 19.17 &  0.32 & 2115.0 &                    O6 & k&         301.4 \\
      HD 171198 &  9.8 & 20.03 & -1.74 & 2173.9 &                   O7: & c&         235.1 \\
    BD-10  4682 &  9.6 & 20.24 &  1.01 & 1979.8 &             O7Vn((f)) & a&         394.3 \\
    BD-11  4674 & 10.2 & 20.98 & -1.22 & 2887.6 &                    O9 & o&         635.3 \\
    HD 175754  & 7.0   & 16.3  & -9.9  & 2181.9 &         O8II(n)((f))p & e &    367.8\\
    HD 175876  & 6.9   & 15.3  &-10.6  & 2463.1 &         O6.5III(n)(f) & e &   240.9\\

\end{longtable}
\begin{minipage}{0.5\textwidth}
\begin{itemize}
\item[a] \cite{2016ApJS..224....4M}
\item[b] \cite{2011ApJS..193...24S}
\item[c] \cite{1988mcts.book.....H}
\item[d]  \cite{1993ApJS...89..293V}
\item[e] \cite{2014ApJS..211...10S} 
\item[f] \cite{2014yCat....1.2023S}
\item[g] \cite{2022AA...657A.131M}
\item[h] \cite{2009MNRAS.400.1479S}
\item[k]   \cite{2003AJ....125.2531R}
\item[o] \cite{1963LS....C04....0N}
\item[l] \cite{1982AJ.....87.1300W} 
\end{itemize}
\end{minipage}

\end{onecolumn}

\begin{onecolumn}
\begin{longtable}{lcccccccc}
\caption{\red{ A list of stars with spectral type OB  from \citet{2003AJ....125.2531R} were their spectral type is found using {\tt Astropy} and {\tt SIMBAD}, and they are limited to the region between $15.5^\circ \leq l \leq 21^\circ$ and  $-5^\circ \leq b \leq 5^\circ$. the stars magnitude  (mag) is listed from \cite{2003AJ....125.2531R} (mag). The distance and using Gaia DR3 parallax \cite{2020yCat.1350....0G} is showed. The distance to the bow-shock is $r$, measured with coordinates given as GL=17.5$^{\circ}$ and GB=$-$5.5$^{\circ}$ \autoref{fig:HII_region}.  Galactic longitude and latitude are $l$ and $b$, respectively.}}  \label{tab:star_photo_fesc2} \\
\toprule
                Name &   $\mathrm{mag}$&  $ {l}$  &    $ {b}$  &     Dist &     S(type) &  S(type) reference &     $r$ &\\
                     &  &  deg    & deg  &  pc$\pm$5\%    &       &        & pc   &  \\
\midrule
\endfirsthead

\toprule
              Name &   $\mathrm{mag}$  & $ {l}$  &    $ {b}$  &   Dist &     S(type) &  S(type) reference &    ${r}$ &      \\
                     &   & deg    & deg  &  pc$\pm$5\%    &       &        & pc  & \\
\midrule
\endhead
\midrule
\multicolumn{8}{r}{{Continued on next page}} \\
\midrule
\endfoot

\bottomrule
\endlastfoot
 LS  IV -12    3 &11.4  &16.23 &  4.88 & 1641.49&           OB- & a &     765.19 \\
     BD-12  4915 & 11.5 &16.81 &  4.35 & 1992.82&            OB & a &     479.4 \\
         LS 4657 & 11.9 &15.57 &  3.49 & 2097.31&           OB+ & a &     400.6 \\
 LS  IV -13    4 & 11.6 &15.60 &  2.93 & 1682.36&           OB- & b &     698.3\\
 LS  IV -14   10 & 11.4 &15.77 &  1.63 & 1751.00&           OB- & b &     616.0\\
     BD-14  4937 & 10.8 &15.60 &  1.49 & 1280.73&           OB- & b &    1056.0\\
     BD-12  4949 & 10.7 &17.17 &  2.32 & 1656.45&            OB & a &     707.6 \\
 TYC 5685-3491-1 & 11.4 &17.89 &  1.93 & 1675.32&            OB & a &     684.1 \\
 LS  IV -13    7 & 11.6 &16.81 &  1.13 & 1680.39&           OB- & b &     669.6\\
     BD-12  4964 & 10.8 &18.11 &  1.80 & 2025.93&            OB & a &     387.6 \\
 LS  IV -14   28 & 11.5 &15.87 &  0.50 & 1520.45&            OB & b &     815.7\\
 LS  IV -12   14 & 11.6 &18.31 &  1.78 & 1920.49&            OB & b &     467.8\\
     BD-12  4975 & 11.1 &18.20 &  1.70 & 1944.39&           OB- & a &     446.8 \\
     BD-12  4977 & 10.7 &18.16 &  1.67 & 2144.08&            OB & b &     311.3\\
     BD-12  4978 & 10.4 &18.24 &  1.70 & 2089.86&            OB & b &     342.7\\
  TYC 5689-418-1 & 10.6 &17.28 &  1.18 & 2055.49&           OB+ & a &     352.1 \\
     BD-12  4982 & 10.1 &18.31 &  1.70 & 2023.88&            OB & a &     386.6 \\
 LS  IV -12   27 & 11.3 &18.39 &  1.73 & 2181.50&            OB & a &     296.7 \\
 LS  IV -14   29 & 11.4 &16.50 &  0.66 & 1631.85&           OB- & b &     709.8\\
 LS  IV -12   32 & 11.0 &17.98 &  1.33 & 1593.62&           OB- & b &     751.9\\
 LS  IV -12   33 & 12.1 &18.48 &  1.59 & 2166.37&           OB+ & a &     298.9 \\
 LS  IV -12   34 & 10.5 &18.58 &  1.60 & 2157.96&           OB- & b &     303.0\\
     BD-12  4994 & 10.6 &18.47 &  1.54 & 2218.27&            OB & a &     277.7 \\
 LS  IV -14   32 & 11.1 &16.29 &  0.34 & 1280.57&           OB- & a &    1045.2 \\
 LS  IV -12   36 & 11.1 &18.01 &  1.25 & 1533.74&           OB- & b &     807.5\\
     BD-12  4996 & 11.5 &18.00 &  1.24 & 2562.13&            OB & a &     365.2 \\
 LS  IV -12   38 & 11.3 &18.09 &  1.25 & 1702.99&           OB- & b &     649.0\\
 LS  IV -12   39 & 11.3 &18.35 &  1.38 & 2198.76&           OB- & a &     278.4 \\
     BD-13  4941 & 10.7 &17.76 &  0.87 & 2099.95&           OB+ & a &     313.5 \\
     BD-12  5008 & 10.8 &18.13 &  1.05 & 1974.33&            OB & a &     409.0 \\
 LS  IV -09    5 & 11.8 &20.87 &  2.44 & 1851.85&           OB- & b &     547.2\\
 LS  IV -14   39 & 11.6 &16.60 & -0.07 & 1940.61&            OB & a &     417.8 \\
 TYC 5689-1271-1 & 11.3 &16.38 & -0.24 & 2351.28&           OB+ & a &     215.5 \\
         LS 4965 & 11.4 &17.18 &  0.12 & 1787.94&           OB- & a &     555.9 \\
  TYC 5689-237-1 & 11.0 &17.20 &  0.07 & 2237.13&           OB+ & a &     223.8 \\
 GSC 06265-01861 & 11.4 &15.53 & -0.82 & 2125.85&            OB & c &     265.7\\
 TYC 6265-2079-1 & 11.0 &15.59 & -0.82 & 1683.21&            OB & c &     648.4\\
 LS  IV -11   16 & 11.9 &19.75 &  1.25 & 1533.74&           OB- & b &     809.8\\
         LS 4992 & 11.2 &17.84 &  0.10 & 1971.99&           OB+ & a &     391.5 \\
 LS  IV -10    7 & 11.7 &20.25 &  1.23 & 1543.92&           OB- & b &     801.5\\
 LS  IV -12   47 & 12.6 &18.88 &  0.44 & 2010.05&           OB- & a &     369.0 \\
     BD-14  5029 & 10.6 &17.23 & -0.44 & 2036.66&            OB & a &     328.5 \\
 LS  IV -13   43 & 11.0 &17.75 & -0.18 & 1560.30&           OB- & a &     767.2 \\
UCAC4 380-107183 & 11.4 &17.25 & -0.46 & 2614.37&           OB- & a &     370.3 \\
 TYC 5702-1189-1 & 11.4 &16.54 & -0.90 & 2040.81&           OB+ & a &     318.7 \\
 LS  IV -14   49 & 11.6 &17.46 & -0.52 & 2297.79&            OB & a &     192.5 \\
 LS  IV -14   50 & 11.7 &16.91 & -0.84 & 1634.78&           OB- & b &     690.3\\
 LS  IV -14   51 & 11.8 &17.49 & -0.62 & 1749.78&           OB- & a &     581.8 \\
         LS 5016 & 11.7 &17.62 & -0.57 & 2554.27&          OB+: & a &     317.7 \\
         LS 5022 & 11.1 &16.10 & -1.49 & 2158.42&           OB+ & a &     222.0 \\
 TYC 5702-1096-1 & 11.4 &18.05 & -0.52 & 1963.09&            OB & a &     387.7 \\
 LS  IV -12   55 & 11.4 &18.68 & -0.19 & 2482.00&           OB: & a &     274.0 \\
UCAC4 384-101260 & 11.5 &18.20 & -0.45 & 2868.61&            OB & a &     600.8 \\
 TYC 5698-3744-1 & 11.5 &18.63 & -0.27 & 2139.03&           OB+ & a &     258.1 \\
     BD-14  5043 & 10.3 &17.06 & -1.15 & 1179.80&            OB & a &    1133.4 \\
 LS  IV -13   45 & 11.4 &18.18 & -0.57 & 2341.92&           OB- & a &     194.6 \\
 LS  IV -15   46 & 10.8 &16.51 & -1.48 & 2675.94&            OB & a &     411.0 \\
 LS  IV -11   19 & 12.1 &20.12 &  0.38 & 2034.58&          OB-e & b &     355.1\\
 LS  IV -15   49 & 11.3 &16.65 & -1.45 & 1906.94&           OB- & b &     426.6\\
 LS  IV -13   46 & 11.6 &17.70 & -0.95 & 2014.91&           OB- & a &     335.5 \\
     BD-14  5048 & 11.6 &16.87 & -1.42 & 2308.40&           OB- & a &     164.9 \\
 LS  IV -14   63 & 11.1 &17.47 & -1.20 & 2302.55&           OB- & a &     168.9 \\
 TYC 5698-4048-1 & 11.4 &18.98 & -0.44 & 2121.79&            OB & a &     266.0 \\
     BD-14  5054 & 10.1 &17.10 & -1.44 & 1591.84&           OB- & b &     726.5\\
     BD-14  5058 &  9.5 &17.77 & -1.15 & 1922.33&           OB- & a &     414.1 \\
 LS  IV -14   71 & 11.4 &17.02 & -1.62 & 2039.15&           OB- & b &     304.4\\
       HD 170061 &  9.9 &17.20 & -1.60 & 1874.76&           OBe & a &     453.1 \\
     BD-13  4990 & 11.0 &18.66 & -0.91 & 2053.81&           OB- & a &     304.7 \\
     BD-16  4894 & 10.4 &15.65 & -2.72 & 1979.41&            OB & a &     350.2 \\
 LS  IV -15   53 & 11.1 &17.05 & -2.01 & 1951.98&           OB- & b &     376.3\\
 LS  IV -12   68 & 11.4 &19.09 & -1.23 & 2331.54&           OB- & a &     173.9 \\
 LS  IV -11   22 & 11.9 &20.39 & -0.61 & 1044.38&           OB- & b &    1272.5\\
     BD-11  4652 & 11.5 &20.27 & -0.77 & 1816.86&           OB- & b &     522.8\\
 LS  IV -12   73 & 12.0 &19.29 & -1.31 & 1719.69&           OB- & b &     604.7\\
 LS  IV -13   59 & 11.7 &18.89 & -1.52 & 2402.11&           OB- & b &     189.6\\
 LS  IV -13   60 & 12.0 &19.02 & -1.48 & 2288.85&           OB- & b &     162.3\\
 LS  IV -13   61 & 11.5 &18.46 & -1.85 & 1817.85&           OB- & b &     503.7\\
 LS  IV -13   67 & 11.2 &18.93 & -1.84 & 1785.39&           OB- & b &     535.7\\
     BD-12  5095 & 10.4 &19.42 & -1.73 & 2146.84&           OB- & a &     219.6 \\
 LS  IV -13   68 & 11.1 &18.85 & -2.05 & 2194.42&           OB- & b &     176.3\\
 LS  IV -12   80 & 11.6 &19.45 & -1.80 & 2602.81&           OB- & b &     340.2\\
     EM* AS  309 & 11.2 &18.54 & -2.42 & 1885.37&          OB-e & b &     433.5\\
 LS  IV -12   83 & 11.7 &19.73 & -1.81 & 2338.08&           OB- & a &     163.1 \\
 LS  IV -13   72 & 10.8 &18.76 & -2.33 & 2160.76&           OB- & a &     191.2 \\
     BD-12  5103 & 11.0 &20.15 & -1.66 & 1459.64&           OB- & b &     857.2\\
 LS  IV -13   74 & 12.0 &18.99 & -2.30 & 1950.07&           OB- & b &     374.6\\
 LS  IV -14   88 & 11.7 &18.25 & -2.70 & 1886.43&           OB- & b &     429.4\\
 LS  IV -14   89 & 11.9 &18.28 & -2.73 & 2173.44&           OB- & b &     170.7\\
     BD-13  5035 & 11.2 &18.88 & -2.55 & 2097.75&           OB- & b &     237.4\\
 LS  IV -12   92 & 11.8 &19.91 & -2.07 & 1301.23&           OB- & b &    1010.4\\
 LS  IV -14   91 & 12.0 &18.45 & -2.83 & 2151.00&           OB- & b &     186.1\\
 LS  IV -11   31 & 11.8 &20.49 & -1.88 & 1479.72&           OB- & b &     837.3\\
 LS  IV -14   94 & 11.9 &18.27 & -3.13 & 2642.70&           OB- & b &     357.2\\
 LS  IV -13   80 & 11.5 &19.63 & -2.80 & 1924.18&           OB- & b &     396.9\\
 LS  IV -14   96 & 11.7 &18.91 & -3.32 & 1751.92&           OB- & b &     556.9\\
 LS  IV -12   96 & 11.6 &19.85 & -2.87 & 1076.77&           OB- & b &    1229.8\\
 LS  IV -11   33 & 11.4 &20.95 & -2.46 & 1751.92&           OB- & b &     571.2\\
 TYC 6271-1204-1 & 11.8 &16.41 & -4.80 & 2962.08&           OB- & a &     665.7 \\
     BD-12  5133 & 11.3 &20.59 & -3.13 & 2794.85&           OB- & a &     513.0 \\
     BD-13  5065 & 10.1 &19.74 & -3.67 & 1872.30&         OB-n: & a &     439.5 \\
         LS 5116 & 12.2 &19.38 & -4.13 & 1787.63&            OB & a &     518.8 \\
 LS  IV -13   86 & 11.7 &19.94 & -3.94 & 1755.92&           OB- & b &     553.0\\
 LS  IV -14  102 & 11.2 &19.06 & -4.69 & 1678.41&           OB- & b &     624.3\\
\end{longtable}
\begin{parallel}
\begin{minipage}{0.5\textwidth}
\begin{itemize}
\item[a]  \cite{1971PWSO...1a...1S}
\item[b] \cite{1963LS....C04....0N}
\item[c]   \cite{2003AJ....125.2531R}
\end{itemize}
\end{minipage}

\end{parallel}

\end{onecolumn}
